# Supplementary material for: Computational design of antimicrobial active surfaces via automated Bayesian optimization
Source: arXiv:2209.00055 source file (2022-08-31)
Supplement: Supplementary file 1 [file SI.tex]

\begin{abstract}
The supplementary information includes additional notes for the mathematical derivation, technical implementations, and additional results in the manuscript. The formulation and parameterization of the empirical potentials are given in Section \ref{para_eqs}. The details and technical implementation of the machine learning potentials are presented in Section \ref{ml_potentials}. The numerical generation of the graphene is proposed and explained in Section \ref{slit}. The numerical experimental design and LAMMPS implementation are also presented. The experimental design for benchmarking the machine learning potentials is given in Section \ref{ml_benchmark_exps}. Supplementary notes on quantized fracture mechanics are given in Section \ref{qfm_theory}. Basic formulation and derivations are presented. Some supplementary discussions on lattice trapping are also given. The characterization and additional results are presented in Section \ref{fracture_characterization}. The details about the implementation in LAMMPS are given in Section \ref{lammps_sec}. Some supplementary discussions are drawn for future directions. If you find any portion of this document helpful, you are encouraged to cite the original article.
\end{abstract}

% {\textbf{\em Keywords:} Biomaterials; Bayesian optimization; machine learning; biofilms; microstructure; individual-based modeling}
%%%%%%%%%%%%%%%%%%%%%%%%%%%%%%%%%%%%%%%%%%%%%%%%%%%%%%%%%%%%%%%%%%%%%
%% Start the main part of the manuscript here.
%%%%%%%%%%%%%%%%%%%%%%%%%%%%%%%%%%%%%%%%%%%%%%%%%%%%%%%%%%%%%%%%%%%%%

\tableofcontents

\section{Empirical Potentials Parameterization\label{para_eqs}}

Although the detailed derivations are already given in the original articles, we provide a basic parameterization of the empirical potentials' equations as a supplementary to perceive the results with a better understanding of theories. The readers should refer to the original publications for full derivations. The goal here is to further explain our simulations and results with the model rather than rederiving everything. Note that the terms are already given in the paper are written in {\sl Tilt Font}, e.g., \textsl{Figure 1}.
% we only present some basic formulations adding to the original equations in our manuscript.
% the full derivations should be referred to the original publications. 

\subsection{Optimized Tersoff}

According to our {\sl Equation (2)} in the article, the potential energy of the Tersoff model writes:\begin{equation}
    V^{\rm\textsc{Tersoff}}_{ij} = f_C (r_{ij}) \left[ A e^{(- \lambda_i r_{ij})} - B_{ij} e^{(-\lambda_2 r_{ij})} \right]\label{opt-tersoff-original_paper}
\end{equation}Here, $A$ is a parameter to be fitted (See Table \ref{opt_tersoff_table}). The second term of $V_{ij}$ represents bonding, where $B_{ij}$ hence includes bond order and depends upon the environment. In the Tersoff formulation, the bonding strength $B_{ij}$ for pair $ij$ follows the form in a simple trial potential \citep{tersoff1986}:
\begin{equation}
    \begin{aligned}
    B_{ij}  = B_0 \mathtt{exp} \left(- \frac{z_{ij}}{b}\right),\\
    z_{ij} = \sum_{k \neq i,j} \left[\frac{w(r_{ik})}{w(r_{ij})} \right]^n \times \left[c + \mathtt{exp}(-d \cos\theta_{ijk}) \right]^{-1}
    \end{aligned}
\end{equation}where $w(r) = f_c(r)\mathtt{exp}(-\lambda_2 r)$, interpreted as the "bare" bonding potential. $z_{ij}$ measures the bonds' numbers competing with bond $ij$. $b$ determines the rate of bond strengths falling off in effective coordination. The final term of $z_{ij}$ proposes the dependence on the angle of potential, where $\theta_{ijk}$ is the angle between bonds $ij$ and $ik$. The Tersoff potential has been modified and applied to study graphene's mechanical, nano-electrical, and vibrational properties of graphene. 

The cutoff function $f_C(r_{ij})$ in Equation (\ref{opt-tersoff-original_paper}) writes\citep{Tersoff_1988}:\begin{equation}
    f^\textsc{Tersoff}_C (r_{ij})  =   \begin{cases}
      1,\ r < R - D\\
      \frac{1}{2} - \frac{1}{2}\sin\left( \frac{\pi}{2} \frac{(r - R)}{D}\right), \ R - D < r < R + D\\
      0, \ r> R + D
    \end{cases}\label{weight}
\end{equation}where $f_C$ is continuous and derivative for all $r$, declining from 1 to 0 in a small range around $R$. Equation (\ref{weight}) tells us that the Tersoff interaction are switched on and off considering the cutoff distances of $R - D$, $R + D$.

In addition to the chi-optimization carried out for the original Tersoff model in {\sl Equation (3)}, the phonon frequencies $\omega_\lambda$ are of greatest focus. The acoustic velocities at the zone center hence write $\Bar{v}_\lambda = \frac{d \omega_\lambda}{d \mathbf{q}}$, where the graphene is in high-symmetry directions. $\lambda = (\mathbf{q}, j)$ attach a phonon with wave vector \textbf{q} in branch $j$. The phonon frequencies are then determined through the calculation carried out in the Brillouin zone. The dynamics matrix writes\citep{opt-tersoff}:\begin{equation}
    D_{\alpha\beta}^{\kappa\kappa'}(\mathbf{q}) = \frac{1}{\sqrt{m_\kappa m_{\kappa'}}} \sum_{\mathbb{L}} \Phi_{\alpha\beta}^{0\kappa,\mathbb{L}'\kappa'}e^{i\mathbf{q}\cdot \mathbf{R}\mathbb{L}'}\label{dynamical_matrix_tersoff}
\end{equation}where $\mathbb{L}_\kappa$ locates the $\kappa$th atom in the $\mathbb{L}$th unit cell. $m_\kappa$ is $\kappa$th atom's mass. $\mathbf{R}_\mathbb{L}$ is the lattice vector for the $\mathbb{L}$th unit cell, where $\alpha$ and $\beta$ are Cartesian components. The parameters implemented in the optimized Tersoff model are shown in Table \ref{opt_tersoff_table}. Note that the symbols for parameterization may differ from different papers, leading to the corresponding mathematical forms possessing different terms. The above derivations are modified and adopted mainly from Refs. \citep{tersoff1986, Tersoff_1988, opt-tersoff, opt_tersoff_2, airebo}

\begin{table}[htbp]
    \centering
    \begin{tabular}{|c|c|c|}\hline
        $A=1.3936\times10^3 eV$ & $B = 3.467\times10^2 eV$ & $\lambda_1 = 3.4879 \mathrm{\text{\AA}}^{-1}$ \\
        $\lambda_2 = 2.2119\mathrm{ \text{\AA}^{-1}}$ & $\lambda_3 = 0.0 \mathrm{\text{\AA}^{-1}}$ & $n = 0.72751$\\
        $c = 3.8049 \times10^4$ & $\beta = 1.5724\times10^{-7}$ & $d = 4.3484$ \\ $\cos\theta_0 = -0.57058$ & $R = 1.95\mathrm{\text{\AA}}$ & $D = 0.15 \mathrm{\text{\AA}}$ \\
        $m = 3$ & $\gamma_{ijk} = 1$& $\ $\\\hline
    \end{tabular}
    \caption{The parameters used in the optimized Tersoff potential \citep{opt-tersoff, opt_tersoff_2}.}
    \label{opt_tersoff_table}
\end{table}

From Equation (\ref{dynamical_matrix_tersoff}) and {\sl Equation (3)} in our paper, we know that the optimization process is mainly concerned with thermal and vibrational properties regarding the mentioned phonon frequencies, acoustic velocities, etc. This also explains the proposition by Si et al. of optimized Tersoff's better accuracy in describing the graphene's thermal properties compared with the other models \citep{potential_model}. 

For the LAMMPS implementation file, a decent example can found at \url{https://github.com/i-pi/i-pi/blob/master/examples/lammps/graphene/C.opt.tersoff}. One can also modify the original Tersoff potential file (a good example is \url{https://github.com/CFDEMproject/LAMMPS/blob/master/potentials/SiC.tersoff}) with the parameters given in Table \ref{opt_tersoff_table}.

A simple implementation in LAMMPS writes:

\begin{lstlisting}[language=c++]
pair_style	tersoff
pair_coeff	* * C.opt.tersoff C
\end{lstlisting}

\subsection{REBO}

Given our provided basic of the REBO formulation in \textsl{Equations (4-5)} in our article, we provide the details of the implemented parameters in the Equations: $w_{ij}$ is a bond-weighting factor\citep{airebo}:\begin{equation}
   f^{\rm REBO}_C (r_{ij})  =   \begin{cases}
      1,\ r < r_{\rm min}\\
      \frac{1}{2}\left[ 1 + \cos \left( \pi \frac{r - r_{\rm min}}{r_{\rm max} - r_{\rm min}}\right)\right], \ r_{\rm min} \leq r < r_{\rm max}\\
      0, \ r \geq r_{\rm max}
    \end{cases}\label{weight_rebo}
\end{equation}
% which switched off long-distance REBO interactions, corresponds to the "switching-off" function we mentioned in the article. The switching function writes:\begin{equation}
%     S' (t) = \Theta (-t) + \Theta (t) \Theta(1-t) \frac{1}{2}[1 + \cos(\pi t)]\label{weight2_eq}
% \end{equation}

% The switching region of different bonds are given by different scaling function, possessing the general form:\begin{equation}
%     t_c (r_{ij}) = \frac{r_{ij} - r_{ij}^{\rm min}}{r_{ij}^{\rm max} - r_{ij}^{\rm min}}\label{weight3_eq}
% \end{equation}

Further details can be found in the Appendix of Ref.\citep{airebo}. In \textsl{Equation (4)}, the bond order term $\Bar{b}_{ij}$ in Abell-Tersoff models follow the term\citep{rebo_deriv_usf}:\begin{equation}
    \begin{aligned}
    \Bar{b}_{ij} = \frac{1}{2} \left(b_{ij}^{\sigma - \pi} + b_{ji}^{\sigma - \pi} \right) + b^{\pi}_{ij}
    \end{aligned}
\end{equation}where\begin{equation}
    b_{ij}^{\sigma - \pi} = \sqrt{1 + \sum_{k \neq i, j} f^{\rm REBO}_C(r_{ik}) g \left(\cos (\theta_{ijk} \right) + P_{ij} (N_i))}
\end{equation}where $b_{ij}^\pi = \Pi_{ij}^{RC} + b_{ij}^{DH}$ is the sum of dihedral and conjugation terms. $g$ is the angular function. $P_{ij}$ is the empirical correction function dependent of carbon configurations $N_i$, written as\begin{equation}
    N_i = \sum_{k \neq i, j}f^{\rm REBO}_C (r_{ik})
\end{equation} The parameters involved in the REBO model are listed in Table \ref{rebo_table_para}.

\begin{table}[htbp]
    \centering
    \begin{tabular}{|c|c|c|}\hline
        $B_1=12 388.791 977 9$eV & $B_2 = 17.567 406 465 0$eV & $B_3 = 30.714 932 080 6$eV \\
        $\beta_1 =  4.720 452 3127$\AA$^{-1}$ & $\beta_2 = 1.433 213 2499$\AA$^{-1}$ & $\beta_3 =  1.382 691 2506$\AA$^{-1}$\\
        $Q = 0.313 460 296 083$\AA & $A =  10 953.544 162 17 $eV & $\alpha= 4.746 539 060 659 $\AA$^{-1}$\\\hline
    \end{tabular}
    \caption{The parameters used in the REBO potential \citep{rebo_deriv_usf}.}
    \label{rebo_table_para}
\end{table}

Example implementation file can be accessed through \url{https://github.com/lammps/lammps/blob/develop/potentials/CH.rebo}. The implementation in LAMMPS writes:

\begin{lstlisting}[language=c++]
pair_style rebo 3.0
pair_coeff * * CH.rebo C
\end{lstlisting}

\subsection{AIREBO}

Based on \textsl{Equation (6)}, we further write AIREBO's nonbonded interactions, which are modeled by a smoothly truncated 12-6 LJ-potential\citep{airebo}:\begin{equation}
    V^{\rm LJ}_{ij} = 4\epsilon_{ij} \left[\left( \frac{\sigma_{ij}}{r}\right)^{12} - \left( \frac{\sigma_{ij}}{r}\right)^{6} \right]
\end{equation}

The energy for LJ interactions from the potential writes:\begin{equation}
    E^{\rm LJ}_{ij} = S(t_r (r_{ij})) S(t_b(b^*_{ij})) C_{ij} V^{\rm LJ}_{ij}(r_{ij}) + [1 - S(t_r (r_{ij}))] C_{ij} V^{\rm LJ}_{ij} (r_{ij})
\end{equation}where $S(t)$ is the switching function\begin{equation}
    S(t) = \Theta (-t) + \Theta (t) \Theta(1-t) [1 - t^2 (3 - 2t)]
\end{equation}where $\Phi(t)$ is the Heaviside step function, and the $S(t)$ function smoothly switches between the values of 0 and 1\citep{rebo_deriv_usf}. The $t$ switches $S$ by employing the dimensionless scaling functions:\begin{equation}
    \begin{aligned}
    t_r (r_{ij}) = \frac{r_{ij} - r_{ij}^{\rm LJ\mathtt{min}}}{r_{ij}^{\rm LJ\mathtt{max}} - r_{ij}^{\rm LJ\mathtt{min}}}, \\
    t_b (b_{ij}) = \frac{b_{ij} - b_{ij}^{\rm LJ\mathtt{min}}}{b_{ij}^{\rm LJ\mathtt{max}} - b_{ij}^{\rm LJ\mathtt{min}}}
    \end{aligned}
\end{equation}

% S(t) = \Theta (-t) + \Theta (t) \Theta(1-t) \frac{1}{2}[1 + \cos(\pi t)]

The torsional potential in \textsl{Equation (6)} writes:\begin{equation}
    V^\textsc{Torsion}(\omega) = \epsilon \left[ \frac{256}{405} \cos^{10}\left( \frac{\omega}{2}\right) - \frac{1}{10}\right]
\end{equation}

The torsional energy hence writes:\begin{equation}
    E^\textsc{Torsion} = \frac{1}{2}\sum_i \sum_{j \neq i} \sum_{k \neq i, j} \sum_{l\neq i, j,k} w_{ij} (r_{ij})w_{jk} (r_{jk}) w_{kl} (r_{kl})\times V^\textsc{Torsion}(\omega_{ijkl})
\end{equation}

The implementation of AIREBO is basically the same as REBO: \url{https://c4science.ch/source/lammps/browse/master/potentials/CH.airebo}. The parameters of the above LJ potential can be found in Ref \citep{rebo_deriv_usf}.

\begin{lstlisting}[language=c++]
pair_style airebo 3.0
pair_coeff * * CH.airebo C
\end{lstlisting}

\subsection{AIREBO-M}

As we already stated in the article, the sole idea of AIREBO-M is to replace the LJ energy in AIREBO with Morse energy for more accurate modeling of carbon-based systems under high pressure. In addition to our original derivation in \textsl{Equations (7-9)}, the parameters in the Morse potential are obtained through fitting location, depth, and second derivative of the potential energy. The fitted maps write\citep{airebo-m}: \begin{equation}
    \begin{aligned}
    \epsilon \longrightarrow \epsilon,\\
    r^{eq} \longrightarrow 2^{\frac{1}{6}}\sigma,\\
    \alpha \longrightarrow 3\times 2^{\frac{5}{6}}\frac{1}{\sigma}
    \end{aligned}
\end{equation}The fitted parameters for C-C interactions write:\begin{table}[htbp]
    \centering
    \begin{tabular}{c|c|c}\hline
        $\epsilon$ (eV) & $\alpha$ (\AA$^{-1}$) & $r^{eq}$ (\AA) \\
        0.0028437 & 1.5722 & 3.8164\\\hline
    \end{tabular}
    \caption{Fitted parameters for AIREBO-M.}
    \label{airebom_tab}
\end{table} 

The implementations basically follow the same for REBO and AIREBO (\url{https://c4science.ch/source/lammps/change/master/potentials/CH.airebo-m}):
\begin{lstlisting}[language=c++]
pair_style airebo/morse 3.0
pair_coeff * * CH.airebo-m C
\end{lstlisting}

\section{Formulation of Machine Learning Potentials\label{ml_potentials}}

Most current state-of-the-art machine learning potentials (MLP), especially neural network potentials, are based on the work of Behler and Parinello\citep{Behler_PRL}. They transform the coordinates (atomic configurations) into a symmetry function that input to the neural network. The symmetry functions include the radial and angular terms. The radial symmetry functions writes:\begin{equation}
    G^R_{i} = \sum_{j\neq i}^{\rm all} e^{-\eta(r_{ij} - r_s)^2} f_C (r_{ij})
\end{equation}and the angular terms write:\begin{equation}
    \begin{aligned}
    G_i^{A} = 2^{1 - \xi} \sum_{j,k\neq i}^{\rm all} (1 + \lambda \cos\theta_{ijk})^\xi \times e^{-\eta(r_{ij}^2 + r_{ik}^2 + r_{jk}^2)} f_C(r_{ij}) f_C(r_{ik}) f_C (r_{jk})
    \end{aligned}
\end{equation}where the angles are $\theta_{ijk} = \frac{\mathbf{R}_{ij}\cdot\mathbf{R}_{ik}}{R_{ij}R_{ik}}$ centered at atom $i$, with $\mathbf{R}_{ij} = \mathbf{R}_i - \mathbf{R}_j$. Other related terms can be referred in Ref.\citep{Behler_PRL}.

Since the focus of our work are not to develop new MLP, but rather to compare existing models for larger-scale simulations employing molecular dynamics methods, the details of the model development are not included in the ESI. Our goal here is to \textbf{outline} the differences of the two models, \textbf{revisit} their core innovations and further \textbf{perceive} the simulation results from the modelling perspective. 

\begin{figure}
    \centering
    \includegraphics[scale=0.25]{img/ml_schematic.pdf}
    \caption{The schematic view for a general machine learning {\em ab initio} potential methods for graphene modeling. Note that the actual details differ from specific models (e.g., for GAP models\cite{gap} and other Gaussian Process Regression-based ML models the approximator/regressor is not a NN anymore); the drawn schematic is the general representation. }
    \label{ML_potential_schematic}
\end{figure}

\subsection{Machine Learning Interatomic Potentials}

The core idea in MLIP is based on the development of moment tensor descriptors. Recall \textsl{Equation (10)}, the basis function $B_\alpha$ is related to the moment tensor descriptors $M$, having the form\citep{mlip}:\begin{equation}
    M_{\mu,\nu}(\mathbf{r}_i) = \sum_j f_\mu (|r_{ij}|, z_i, z_j) \underbrace{\mathbf{r}_{ij} \otimes ... \otimes \mathbf{r}_{ij}}_{\nu\ \rm times}
\end{equation}where $f_\mu$ stands for the radial part we previously mentioned, writes\begin{equation}
    f_\mu (|r_{ij}|, z_i, z_j) = \sum_{\beta=1}^{N_Q} c_{\mu, z_i, z_j}^{(\beta)} Q^{(\beta)}(|r_{ij}|),
\end{equation}where $\mathbf{c} = \{c_{\mu, z_i, z_j}^{(\beta)}\}$ include the parameters for the radial functions. $Q^{(\beta)}(|r_{ij}|)$ are referred as the radial basis function\begin{equation}
    Q^{(\beta)}(|r_{ij}|)  =   \begin{cases}
      \phi^{(\beta)} (|r_{ij}|) \left(r_{\rm max} - |r_{ij}|\right)^2,\ |r_{ij}| < r_{\rm max}\\
      0, \ |r_{ij}| \geq r_{\rm max}
    \end{cases}
\end{equation}where $\phi^{(\beta)}$ are polynomial functions on the intervals between $[r_{\rm min}, r_{\rm max}]$. Consider our schematic illustration in Figure \ref{ML_potential_schematic}, the radial part are based on the upper-left zoomed view:\begin{equation}\mathbf{r}_{ij}\otimes\mathbf{r}_{ij} = 
    \begin{bmatrix}
    x_{ij}^2 & x_{ij}y_{ji} & x_{ij}z_{ij}\\
    y_{ij}x_{ij} & y^2_{ij} & y_{ij}z_{ij}\\
    z_{ij}x_{ij} & z_{ij}y_{ij} & z^2_{ij}
\end{bmatrix}
\end{equation}Now going back to our initial point, the basis functions are related to the moment tensor descriptors in the form of\begin{equation}
    \begin{aligned}
    B_1 &= M_{0,0},\quad
    &B_2 &= M_{1,0},\quad
    &B_3 &= M_{0,0}^2,\\
    B_4 &= M_{0,1}\cdot M_{0,1},\quad
    &B_5 &= M_{0,2}: M_{0,2},\quad
    &B_6 &= M_{0,0}M_{1,0},\\
    B_7 &= M_{0,0}^3,\quad
    &B_8 &= M_{0,0}(M_{0,1}\cdot M_{0,1}),\quad
    &B_9 &= M_{0,0}^4.
    \end{aligned}
\end{equation}where the level of $M_{\alpha,\beta}$ are defined to assign certain values for exact implementations, i.e., ${\rm lev}{M_{\mu,\nu}} = 2 + 4\mu + \nu$, which we can further derive the value of ${\rm lev}_{i = 1,...,9}B_i$. The details are given Ref\citep{mlip}. Here, the training parameters we wrote in \textsl{Equation (11)} in the article contains the parameters of both angular and radial parts: $\theta = \{ \xi, \mathbf{c} \}$.

\subsection{Dropout Uncertainty Neural Network Potentials}

\textsl{Equations (12 - 14)} constitutes the DUNN through eliciting dropout matrices \textbf{D}. The training of DUNN follows what is given in \textsl{Equation (11)}. The difference is the loss in DUNN contains only MSE of the energies and forces, multiplies the weighted factors\citep{dunn},\begin{equation}
    \mathcal{L} = \sum_{m=1}^M \frac{1}{2} w_m^e \left[ E (\mathbf{r}_m; \theta ) - E_m^{\rm DFT}\right]^2 + \sum_{m=1}^M \frac{1}{2} w_m^f \left|\left|\mathbf{f} (\mathbf{r}_m; \theta ) - \mathbf{f}_m^{\rm DFT}\right|\right|^2
\end{equation}where $E (\mathbf{r}_m; \theta )$ is the energy approximated via the DUNN. The force can then be obtained via computing the derivative $\mathbf{f} (\mathbf{r}_m; \theta ) = -\frac{\partial E}{\partial \mathbf{r}}|_{\mathbf{r}_m}$ are the concatenated forces from the configuration $m$. The weights of the energy and forces are set to be\begin{equation}
    w_m^e = \frac{1}{N_m^2},\quad w_m^f = \frac{1}{10 N_m^2}
\end{equation}The weight of energy $w_m^e$ is assigned to ensure a normalization for roughly equally contribution by each atomic configuration. The normalization in the force weight $w_m^f$ was to make each force component have roughly the same contributions in the training processes.

The detailed implementation of DUNN can be found in Ref.\citep{dunn}. Here, we mainly adopt the ``{\em Supplementary Note}" of Wen and Tadmor\citep{dunn} to give our general perspective of their model, and how we perceive the phenomena observed based on the mathematics in the model. The goal here is not to rewrite everything, but rather to explain the formulation for a better understanding of our simulations and further discussions.

\subsection{Applications in LAMMPS}

The implementation of MLIP was rather simple. One simply replace the original \texttt{pair\_style} command: 
\begin{lstlisting}[language=c++]
pair_style      mlip mlip.ini
pair_coeff		* *
\end{lstlisting}

Based on our practices, the way we would recommend to install MLIP is: (1) download and compile \texttt{mlip} model through \texttt{gitlab}; (2) \texttt{mlip-lammps-interface} should better be installed before \texttt{lammps}; (3) install a stable version of \texttt{lammps} and compiled this one separately with \texttt{make yes-user-mlip}; then one can follow their preferred way to compile LAMMPS, either with \texttt{make mpi} under \texttt{src} or via CMAKE through building a \texttt{build} directory.

The implementation of DUNN(s) is enabled through the \texttt{openkim} library. Install \texttt{openkim} and \texttt{kim-api} is a bit complicated if one don't have the \texttt{sudo} access, e.g., if one uses a supercomputer (SC) with limited permissions. A good way to bypass this issue is to specify the C++ route in the SC environment for targeted compiling. Or simply contact for service assistance. After \texttt{openkim} is successfully installed, one may also need to pay attention to the \texttt{wget} of the computer system. Note that \texttt{openkim} may not favor specific version of \texttt{wget}, e.g., the one in Stampede2. A good way to solve this is to download \texttt{wget} via through \texttt{Anaconda}.

To implement the OpenKIM potential, one needs to first replace the original field:
\begin{lstlisting}[language=c++]
units metal
\end{lstlisting}
to 
\begin{lstlisting}[language=c++]
kim_init DUNN_WenTadmor_2019v2_C__MO_956135237832_000 metal
\end{lstlisting}
and hence replace all the \texttt{pair\_style} and \texttt{pair\_coeff} to a single line:
\begin{lstlisting}[language=c++]
kim_interactions C
\end{lstlisting}

where \texttt{DUNN\_WenTadmor\_2019v2\_2\_\_MO\_956135237832\_000} should be the potential model you wish to apply and findable in the OpenKIM database.

% As we have already written in the article, 

% The differences of 

% \subsection{Possible Technical Issues}

% In our attempts, many issues arise from the underlying version of C++. Herein listed a few possible issues when installing.

% \begin{itemize}
%     \item The preinstallation of \texttt{kim-api} may cause some issues implemented in some supercomputer environments. Assume most peopSpecify the C++ interpreter
%     \item Some versions of \texttt{openkim} may not favor some specific version of \texttt{wget}.
%     \item The correct way to install MLIP model: (1) \texttt{mlip} model (2) \texttt{mlip-lammps-interface} should better be installed before \texttt{lammps}.
% \end{itemize}

% For fast and easy implementation, we also provide a bash file to install the MLIP model

\section{Graphene Slit\label{slit}}

\subsection{Backgrounds}

A graphene slit is usually considered unavoidable during the manufacturing process considering the atom layer is so thin even the slightest nano-equipment can cause trivial damage. Graphene slit are also widely used in water desalination, where the small pore allows only certain numbers of water molecules to transport. In fracture mechanics, such slit (or defect) are adopted to be considered as a precrack for us.
% This is reported in the work of 

\subsection{Numerical Representation}

One should not simply remove atoms form the graphene sheet to create the vacancy. Rather, removing a single carbon atom causes bond reformation, leading to other types of defects such as Stone-Wales defect, Jahn-Teller distortion, etc. Here, we create the vacancy based on the work of Zhao and Aluru \citep{jap} shown in Figure \ref{vacancy}. The double vancacy is firstly created via removing the connected two red atoms in Figure \ref{vacancy}, which should not cause additional bonds to formulate. Then the adjacent carbon atoms indicated in blue are hence removed. The combined red and blue carbon atoms can be considered as a vacancy unit. The defect is created via continuously creating such defects.

\begin{figure}
    \centering
    \includegraphics[scale=0.25]{img/vacancy_explain.pdf}
    \caption{Schematic illustration of the creation of the initial defect, or a graphene slit. The connected red carbon atoms indicate a double-vacancy, with their adjacent blue atoms continuously removed. The crack length (or initial defect length) $L_C$ is calculated based on the longest distance between armchair carbon bonds. The width (0.71nm) is computed as the longest distance of the zigzag carbon atoms.}
    \label{vacancy}
\end{figure}

\section{Benchmarking Machine Learning Potentials\label{ml_benchmark_exps}}

\subsection{Experimental Design}

Mainly concerned with the slow computation process, we scale down the system in size. A smaller simulation box with widths of each side of approximately 10nm and a height of 6nm is set as shown in Figure \ref{smallbox}. The computational procedure remains the same, in which details are to be explained in Section \ref{lammps_sec}.

\begin{figure}
    \centering
    \includegraphics[scale=0.42]{img/smallbox_schematic.pdf}
    \caption{Schematic view for the generation of the small box simulation for benchmarking the DUNN machine learning potentials. A smaller box with a similar setup of defected graphene sheet of width and length of $\sim$10nm is indicated on the right.}
    \label{smallbox}
\end{figure}

\subsection{Results of MLIP}

The full simulation results are shown in Figure \ref{ml}, where details can be referred to in the captions. It is observed that the stress concentration phenomena are too evident. Brittle fracture is observed. The general fracture processes do not exhibit much differences.

\begin{figure}
    \centering
    \includegraphics[scale=0.3]{img/ml_full.pdf}
    \caption{The full graphene fracture process with small initial defect under four different temperature gradients (i.e., 0K, 100K, 200K, 300K) are illustrated in the four subfigures {\bf A} to {\bf D}. The corresponding strains of each moment are marked on top. The virial atomic stresses in X direction are in bar-$\rm\AA^3$.}
    \label{ml}
\end{figure}

\section{Quantized Fracture Mechanics\label{qfm_theory}}

QFM is a modification of continuum mechanics employing discrete perspectives. The calculation relates to continuum theories via the stress intensity from linear elastic fracture mechanics derived from Griffith's theory.

\subsection{Derivation from Continuum Mechanics}

The energy release rate in fracture is defined as\begin{equation}
    G = \frac{K_I^2}{E'} + \frac{K_{II}^2}{E'} + \frac{1 + \nu}{E} K_{III}^2
\end{equation}where $K_{I,II,III}$ are fracture intensities of mode I, II, III cracks. For plane stress, $E' = E$; for plane strain, $E' = \frac{E}{1 - \nu^2}$. The basic formulation of LEFM follows\citep{qfm}:\begin{equation}
    \begin{aligned}
        G \equiv -\frac{dW}{dA} = G_C;\quad \left(\frac{d G}{dA} \right)_C < 0\ \longrightarrow \rm stable,\quad if >0\ \longrightarrow \rm LEFM\\
        K_{I, II, III} = K_{I, II, III C}; \quad \left(\frac{d K_{I,II,III}^2}{dA} \right)_C < 0\quad \longrightarrow \rm stable,\ if >0\ \longrightarrow \rm LEFM\label{lefm}
    \end{aligned}
\end{equation}$W$ is the total potential energy. $C$ denotes the critical condition in crack propagation. Now, recall that QFM assumes additional discrete crack propagation over Griffith's criterion, if we replace all the differentials in Equation (\ref{lefm}) into finite differences with difference $\Delta$, the above equation can be rewrite into:\begin{equation}
    \begin{aligned}
        G \equiv -\frac{\Delta W}{\Delta A} = G_C;\quad \left(\frac{\Delta G}{\Delta A} \right)_C < 0\ \longrightarrow \rm stable,\quad if >0\ &\longrightarrow \rm QFM\\
        K^{\star}_{I, II, III} = \sqrt{\langle K^2_{I, II, III} \rangle_A^{A + \Delta A}} = K_{I, II, III C}; \quad \left(\frac{\Delta K^{\star2}_{I,II,III}}{\Delta A} \right)_C < 0\quad &\longrightarrow \rm stable,\\ \rm if >0\ &\longrightarrow \rm QFM\label{qfm_eqn}
    \end{aligned}
\end{equation}where the term $\langle\rangle_A^{A+\Delta A}\equiv \frac{1}{\Delta A} \int_{A}^{A + \Delta A} dA$. If $\Delta A$ is defined as a fracture quantum, the dissipation energy in QFM is $G_C\Delta A$.

\subsection{Derivation for Fracture Stress}

The derivation of the fracture stresses start by assuming a Griffith's case of a linear elastic infinite plate under tension with thickness $t$, of the precrack $L_C = 2\mathfrak{L}$ under a mode I loading. The prediction of the fracture stresses by LEFM and QFM are\begin{equation}
    \sigma_{\rm LEFM}(\mathfrak{L}) = \frac{K_{IC}}{\sqrt{\pi \mathfrak{L}}},\quad \sigma_{\rm QFM}(\mathfrak{L}) = \frac{K_{IC}}{\sqrt{\pi(\mathfrak{L} + \frac{L_0}{2})}}
\end{equation}Here, $L_0 \approx \frac{2K_{IC}^2}{\pi \sigma_C^2}$, where $\sigma_C$ is the materials strength. In this case, interestingly, the LEFM and QFM predicted crack propagations are unstable. If one extend the brittle fracture to a blunt one, the fracture stress are then given the form we derived in \textsl{Equation (17)}, further expanded in the form:\begin{equation}
    \sigma_\mathcal{F} (\mathfrak{L}, \rho) = K_{IC} \sqrt{\frac{1 + \frac{\rho}{2L_0}}{\pi (\mathfrak{L} + \frac{L_0}{2})}} = \sigma_C \sqrt{\frac{1 + \frac{\rho}{2L_0}}{1 + \frac{2\mathfrak{L}}{L_0}}}\label{frac_strss}
\end{equation}with most of the parameters have already been explained in the article. A full and detailed derivation can be found in Ref.\citep{qfm}. We only extract the portion useful for our work.

\subsection{Supplementary Discussion on Thermal Activation}

Another interesting point we want to emphasis here is the thermal activation as driving to initialize the damage. Extending Equation (\ref{frac_strss}) to the scenario of the plate with a limited width, Anderson \citep{Anderson_frac_mech_book} proposed the form of fracture stress:\begin{equation}
    \sigma_\mathcal{F} (\mathfrak{L}) = \sigma_C (\dot{\epsilon}, T)\sqrt{\frac{1 + \frac{\rho}{2L_0}}{1 + \frac{2\mathfrak{L}}{L_0}}} \left[ \frac{2w}{\pi \mathfrak{L}} \tan\left(\frac{\pi \mathfrak{L}}{2w}\right)\right]^{\frac{1}{2}}
\end{equation}where $2w$ is the width of the plate. Now, to determine the fracture stress using this form, one should calculate $\sigma_C$, which is interpreted as the critical stress, i.e., the strength of the pristine (defect-free) graphene. 

Note that $\sigma_C = \sigma_C (\dot{\epsilon}, T)$, is highly dependent on strain rate and temperatures. Analytically, one could determine $\sigma_C$ through fracture kinetic analysis, following the form given by Zhao and Aluru \citep{jap}. Regarding {\sf thermal activation}, applying the theorem by Eyring \citep{eyring}, the life time $\tau$ relates to tensile stress $\sigma$ and temperature $T$ in a relation of \begin{equation}
    \tau = \frac{\tau_0}{n_s} \exp\left(\frac{U_0 - \gamma\sigma}{kT}\right)\label{thermal_act}
\end{equation}By substituting Equation (\ref{thermal_act}) and apply damage criterion that relates $\tau$ to $t$, one could obtain the analytical form of $\sigma_C$. From this $\sigma_C$ one could also fit the MD simulation data.

% We would like Prof. Derek Warner on raising the question that pushes towards this section.

\section{Fracture Characterizations\label{fracture_characterization}}

Figure \ref{contour} shows the 3D contour visualization corresponds to the \textsl{Figure 4} in the manuscript. The white dots indicate the scattered points from the MD simulations. The contour provide a decent perception of how the fracture stresses and strains are randomly correlated with the temperature gradients.

\begin{figure}[htbp]
    \centering
    \includegraphics[scale=0.65]{img/yield_fracture_profile.pdf}
    \caption{The contour plot for yield stresses $\sigma_Y$ and the corresponding yield strain $\epsilon_Y$ with respect to precrack lengths $L_C$ and thermal gradients $\rm \Delta T$. In the left subfigure, each black dashed line stands for a gradient value of 5; in the right subfigure, each black dashed line stands for a gradient value of 0.5.}
    \label{contour}
\end{figure}

\begin{figure}
    \centering
    \includegraphics[scale=0.3]{img/SI_REBO.pdf}
    \caption{The full initial fracture graphical representation of different initial defect lengths, temperature gradients under the REBO potential. The arrows marked the fracture propagation direction. Note that an unobvious initial fracture yet with specific directional trend observed is marked with a double arrow with the crack propagation direction marked with deep gray. The virial atomic stress are represented accroding to the color bar, in the units of bar-$\rm\AA^3$.}
    \label{rebo}
\end{figure}

\begin{figure}
    \centering
    \includegraphics[scale=0.3]{img/SI_AIREBO.pdf}
    \caption{The full initial fracture graphical representation of different initial defect lengths, temperature gradients under the AIREBO potential. The arrows marked the fracture propagation direction. Note that an unobvious initial fracture yet with specific directional trend observed is marked with a double arrow with the crack propagation direction marked with deep gray. The virial atomic stress are represented accroding to the color bar, in the units of bar-$\rm\AA^3$.}
    \label{airebo}
\end{figure}

\begin{figure}
    \centering
    \includegraphics[scale=0.3]{img/SI_AIREBOM.pdf}
    \caption{The full initial fracture graphical representation of different initial defect lengths, temperature gradients under the AIREBO-M potential. The arrows marked the fracture propagation direction. Note that an unobvious initial fracture yet with specific directional trend observed is marked with a double arrow with the crack propagation direction marked with deep gray. The virial atomic stress are represented accroding to the color bar, in the units of bar-$\rm\AA^3$.}
    \label{airebom}
\end{figure}

\begin{figure}
    \centering
    \includegraphics[scale=0.3]{img/SI_OptTersoff.pdf}
    \caption{The full initial fracture graphical representation of different initial defect lengths, and temperature gradients under the optimized Tersoff potential. The arrows marked the fracture propagation direction. Note that an unobvious initial fracture yet with a specific directional trend observed is marked with a double arrow with the crack propagation direction marked with deep gray. The virial atomic stress is represented according to the color bar, in the units of bar-$\rm\AA^3$.}
    \label{opttersoff}
\end{figure}

\begin{table}[htbp]
    \centering
    \begin{tabular}{c|c c c c c c}
        \texttt{AIREBO} & $L_C$ (nm) & 1.7217 &  $3.1974$ & $ 4.1812$ & $5.6569$ & $ 8.1164$ \\\hline
        $\Delta {\rm T} = 0$K & & \cmark & \cmark & \cmark & \cmark & \cmark\\
        $\Delta {\rm T} = 100$K & &  \xmark & \xmark & \xmark & \xmark & \cmark \\
        $\Delta {\rm T} = 200$K & &  \cmark & \cmark & \xmark & \xmark & \xmark \\
        $\Delta {\rm T} = 300$K & &  \xmark & \cmark & \cmark & \cmark & \cmark \\\hline
        \texttt{REBO} & $ L_C$ (nm) & 1.7217 & $ 3.1974$ & $ 4.1812$ & $ 5.6569$ & $ 8.1164$ \\\hline
        $\Delta {\rm T} = 0$K & & \xmark & \xmark & \xmark & \cmark & \xmark \\
        $\Delta {\rm T} = 100$K & & \xmark & \xmark & \xmark & \xmark & \xmark\\
        $\Delta {\rm T} = 200$K & & \xmark & \xmark & \cmark & \cmark & \cmark \\
        $\Delta {\rm T} = 300$K & & \xmark & \xmark & \xmark & \cmark & \xmark\\\hline
        \texttt{Opt-Tersoff} & $L_C$ (nm) & 1.7217 & $ 3.1974$ & $ 4.1812$ & $5.6569$ & $ 8.1164$ \\\hline
        $\Delta {\rm T} = 0$K & & \xmark & \xmark & \xmark & \xmark & \xmark\\
        $\Delta {\rm T} = 100$K & & \xmark & \xmark & \xmark & \xmark & \xmark \\
        $\Delta {\rm T} = 200$K & & \xmark & \xmark & \xmark & \xmark & \xmark  \\
        $\Delta {\rm T} = 300$K & & \xmark & \xmark & \xmark & \xmark & \xmark\\\hline
        \texttt{AIREBO-M} & $ L_C$ (nm) &  1.7217 & $ 3.1974$ & $ 4.1812$ &  $ 5.6569$ & $ 8.1164$ \\\hline
        $\Delta {\rm T} = 0$K & & \xmark & \xmark & \xmark & \xmark & \xmark \\
        $\Delta {\rm T} = 100$K & & \xmark & \xmark & \xmark & \xmark & \xmark\\
        $\Delta $ T = 200K & & \xmark & \cmark & \cmark & \cmark & \xmark \\
        $\Delta $ T = 300K & & \xmark & \xmark & \xmark &  \cmark & \cmark \\\hline
    \end{tabular}
    \caption{The recordings of the anomalous fracture under different conditions.}
    \label{table_direction}
\end{table}

Table \ref{table_direction} shows the recording of whether the anomalous kinetic energy transportation happens. The results are further discussed in the article.

Figures \ref{rebo}-\ref{opttersoff} shows the initial crack propagation of different initial cracks under different temperature gradients by employing REBO, AIREBO, AIREBO-M, and optimized Tersoff, respectively.

\section{LAMMPS Implementation\label{lammps_sec}}

Herein attached is a simple explanation of our implementations in LAMMPS. Those who may be interested in implementing our code are welcome to contact any of the authors to require the necessary code \& data.

One first setup the simulation box:
\begin{lstlisting}[language=c++]
clear 
units metal
dimension 3 
boundary p p p 
atom_style atomic
\end{lstlisting}
Read the data of the modeled system (can be generated from VMD, nanohub, etc.)
\begin{lstlisting}[language=c++]
read_data   graphene_model.data
mass 1 12.0107
\end{lstlisting}

Define the interatomic potentials. Here we use the simplest REBO for example. \footnote{This step is essential in our works.}
\begin{lstlisting}[language=c++]
pair_style rebo 3.0
pair_coeff * * CH.rebo C
\end{lstlisting}

Systems configurations, initial temperature setup, convergence properties setup.

\begin{lstlisting}[language=c++]
neighbor 2.0 bin 
neigh_modify every 1 delay 0 check yes
velocity all create 300.0 63457 mom yes rot yes dist gaussian
timestep        0.0005
thermo          1000
fix 1 all box/relax x 0.0 y 0.0
minimize 1.0e-8 1.0e-12 1000 10000
\end{lstlisting}

Define the regions and setup the geometries:
\begin{lstlisting}[language=c++]
region all block INF INF INF INF INF INF units box

variable bottom equal bound(all,ymin,all)
variable top equal bound(all,ymax,all)
variable b_width equal ${bottom}+5
variable t_width equal ${top}-5
variable heat_width equal ${b_width}+100
variable cool_width equal ${t_width}-100

region border1 block INF INF INF ${b_width} INF INF units box
region border2 block INF INF ${t_width} INF INF INF units box
region heat block INF INF ${b_width} ${heat_width} INF INF units box
region cool block INF INF ${cool_width} ${t_width} INF INF units box

group border1 region border1
group border2 region border2
group boundary union border1 border2
group heat region heat
group cool region cool 
group interior subtract all boundary 
\end{lstlisting}

Run for equilibration, as we mentioned in the article:
\begin{lstlisting}[language=c++]
reset_timestep 0
fix 2 interior nve
fix 3 heat heat 1 50.0 region heat
fix 4 cool heat 1 -50.0 region cool
run 10000
\end{lstlisting}

Setup parameters for tensile loadings:
\begin{lstlisting}[language=c++]
compute peratom all pe/atom
compute strs all stress/atom NULL pair virial
compute kitc all ke
compute tempa all temp
compute fcom all reduce sum c_strs[1]
variable sigma equal c_fcom

thermo_style custom step temp pe lx ly lz press pxx pyy pzz 
\end{lstlisting}

Apply the tensile loading for fractures
\begin{lstlisting}[language=c++]
reset_timestep	0

variable srate equal 1.0e10
variable srate1 equal "v_srate / 1.0e12"
fix		tens all deform 1 x erate ${srate1} units box remap x

thermo_style	custom step v_strain temp v_p2 v_p3 v_p4 ke pe press

run		50000
\end{lstlisting}

Collect data for post-processing (nomenclature may differs from case to case)
\begin{lstlisting}[language=c++]
variable strain equal "(lx - v_L0)/v_L0"
variable p1 equal "v_strain"
variable p2 equal "-pxx*0.0001"
variable p3 equal "-pyy*0.0001"
variable p4 equal "-pzz*0.0001"
variable tp equal "temp"

fix def1 all print 100 "${p1} ${p2} ${sigma} ${tp}" file crack1_0.txt screen no

dump 		2 all custom 100 crack1_0.dump mass type xs ys zs vx vy vz fx fy fz c_strs[1] c_strs[2] c_strs[3]
dump_modify 2 element C
\end{lstlisting}

$^\star$Note that the steps listed herein are only the key steps. The readers can adopt the basic ideology and readjust based on their own systems.

% \section*{Acknowledgement}

% We thank Prof. Derek Warner for additional discussions regarding the fracture mechanics of graphene.

% \bibliography{new}
% \end{document}
